# Supplementary material for: Pose-Controllable Talking Face Generation by Implicitly Modularized Audio-Visual Representation
Source: arXiv:2104.11116 source file (2021-04-22)
Supplement: Supplementary file 1 [file additional.pdf]

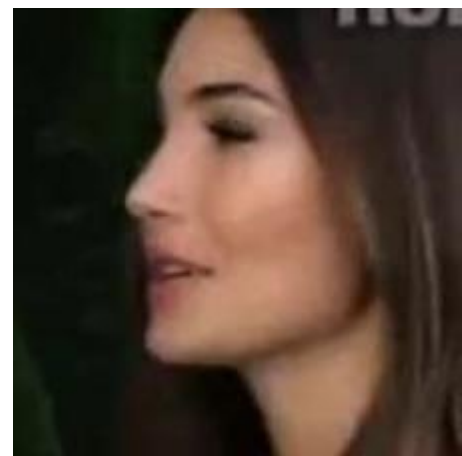

**Identity  
Reference**

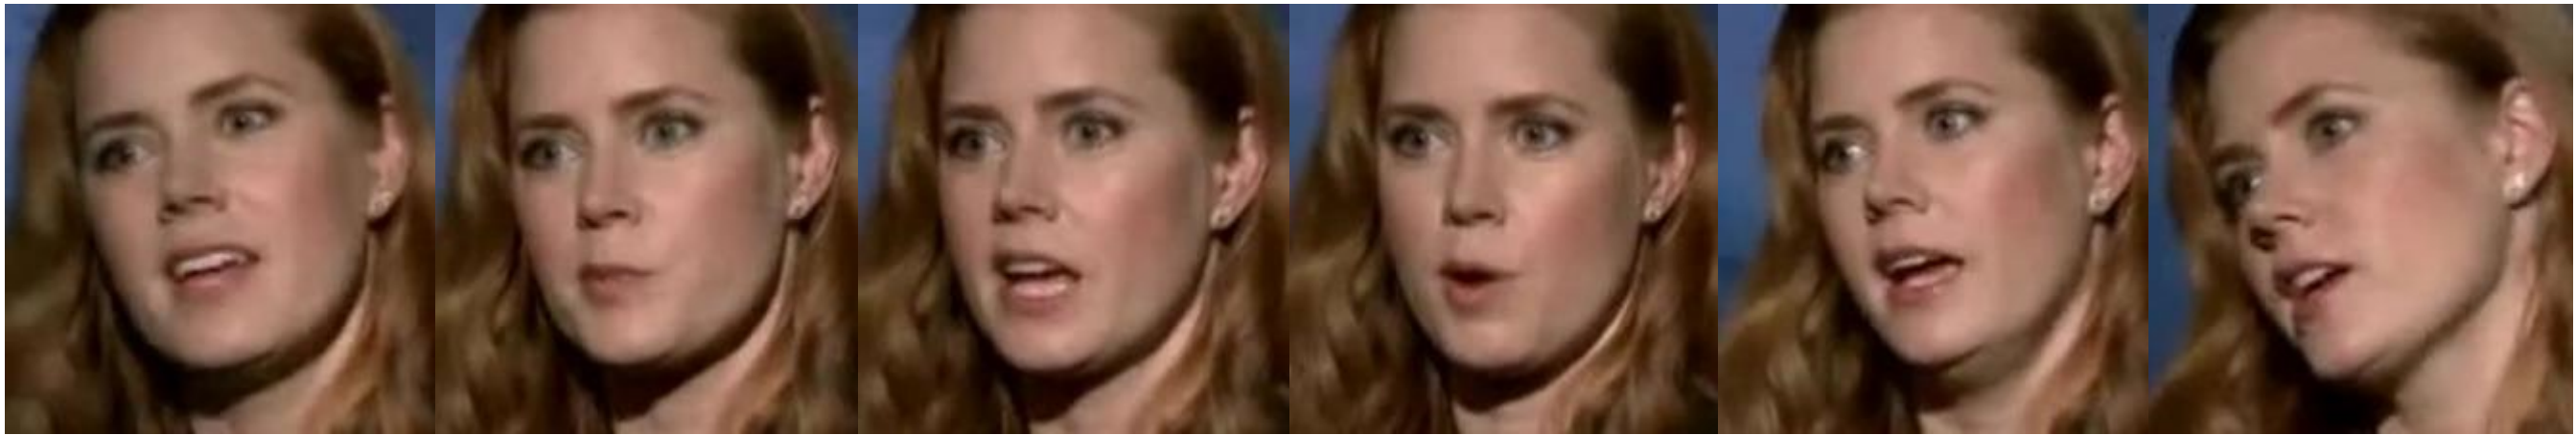

**Synced  
Video**

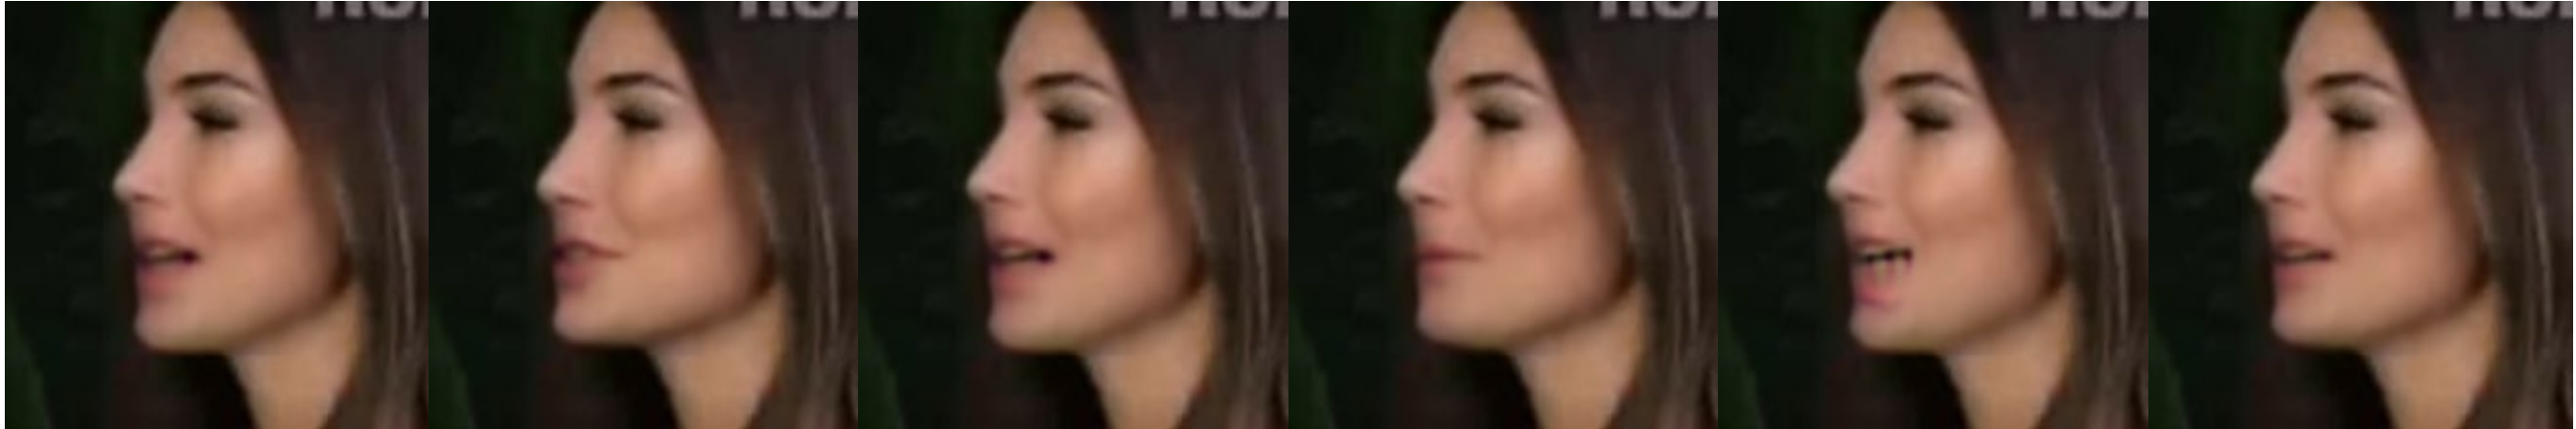

**Wav2Lip**

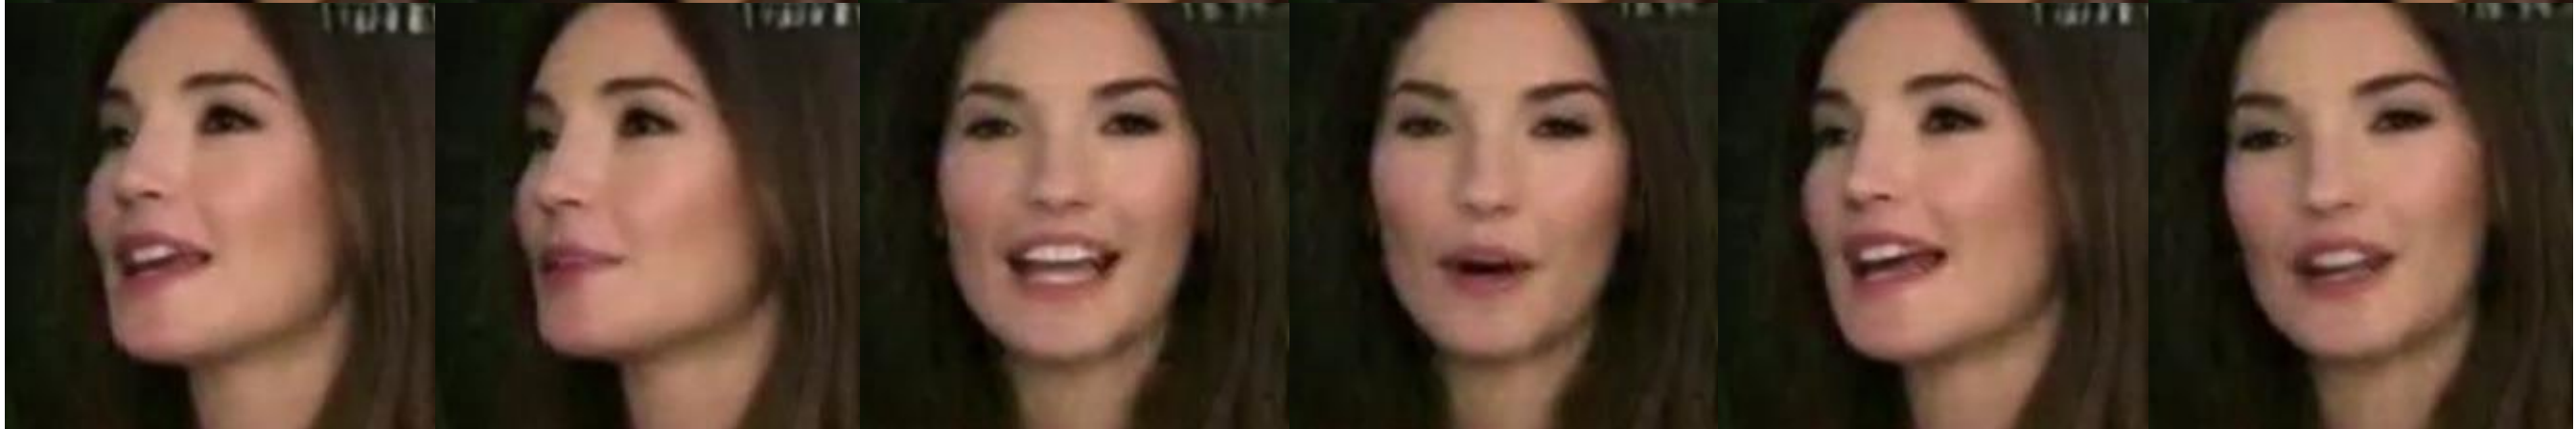

**Ours**

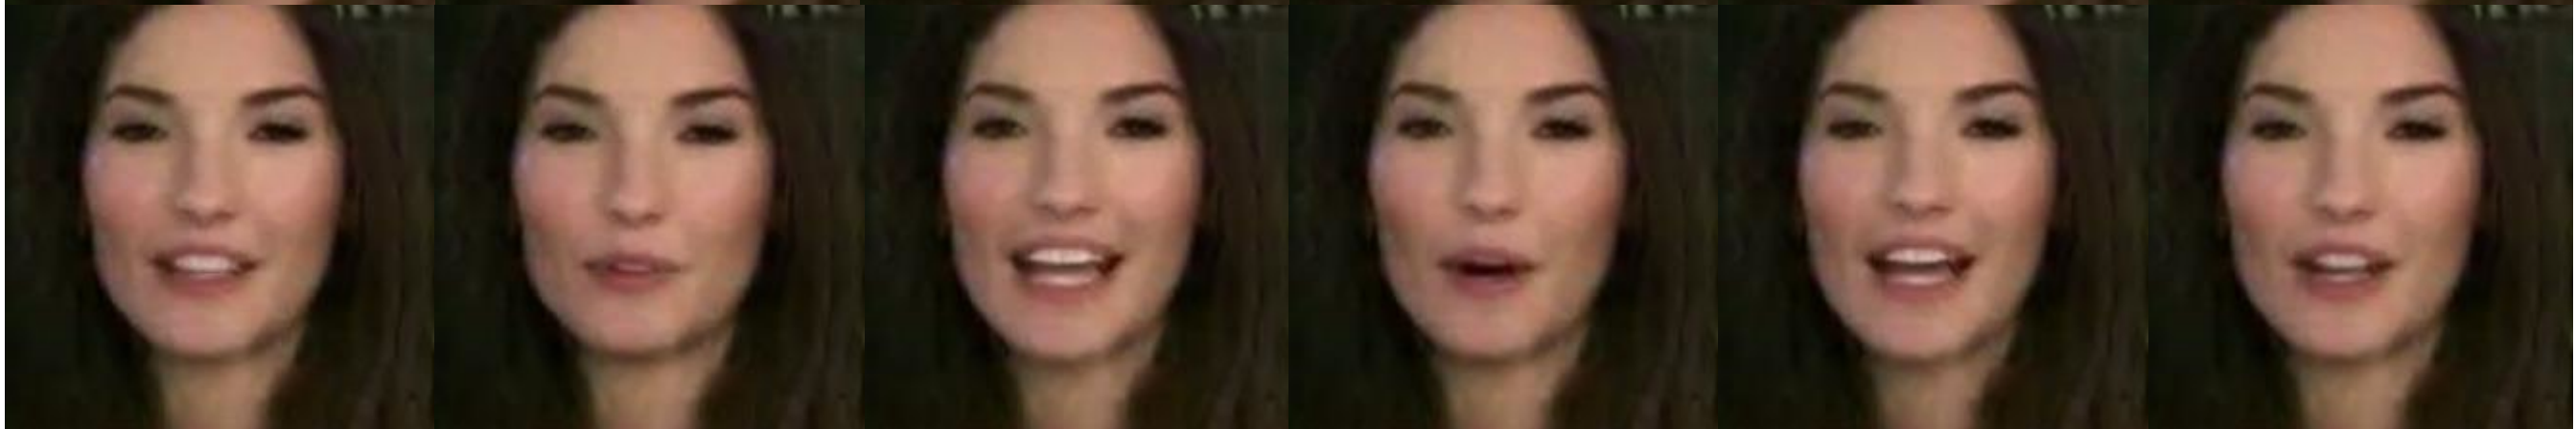

**Frontalized**



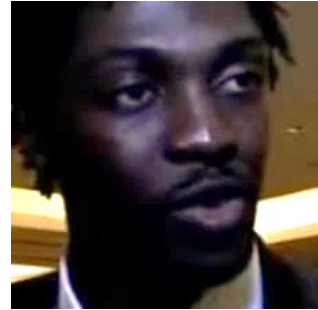

Identity  
Reference

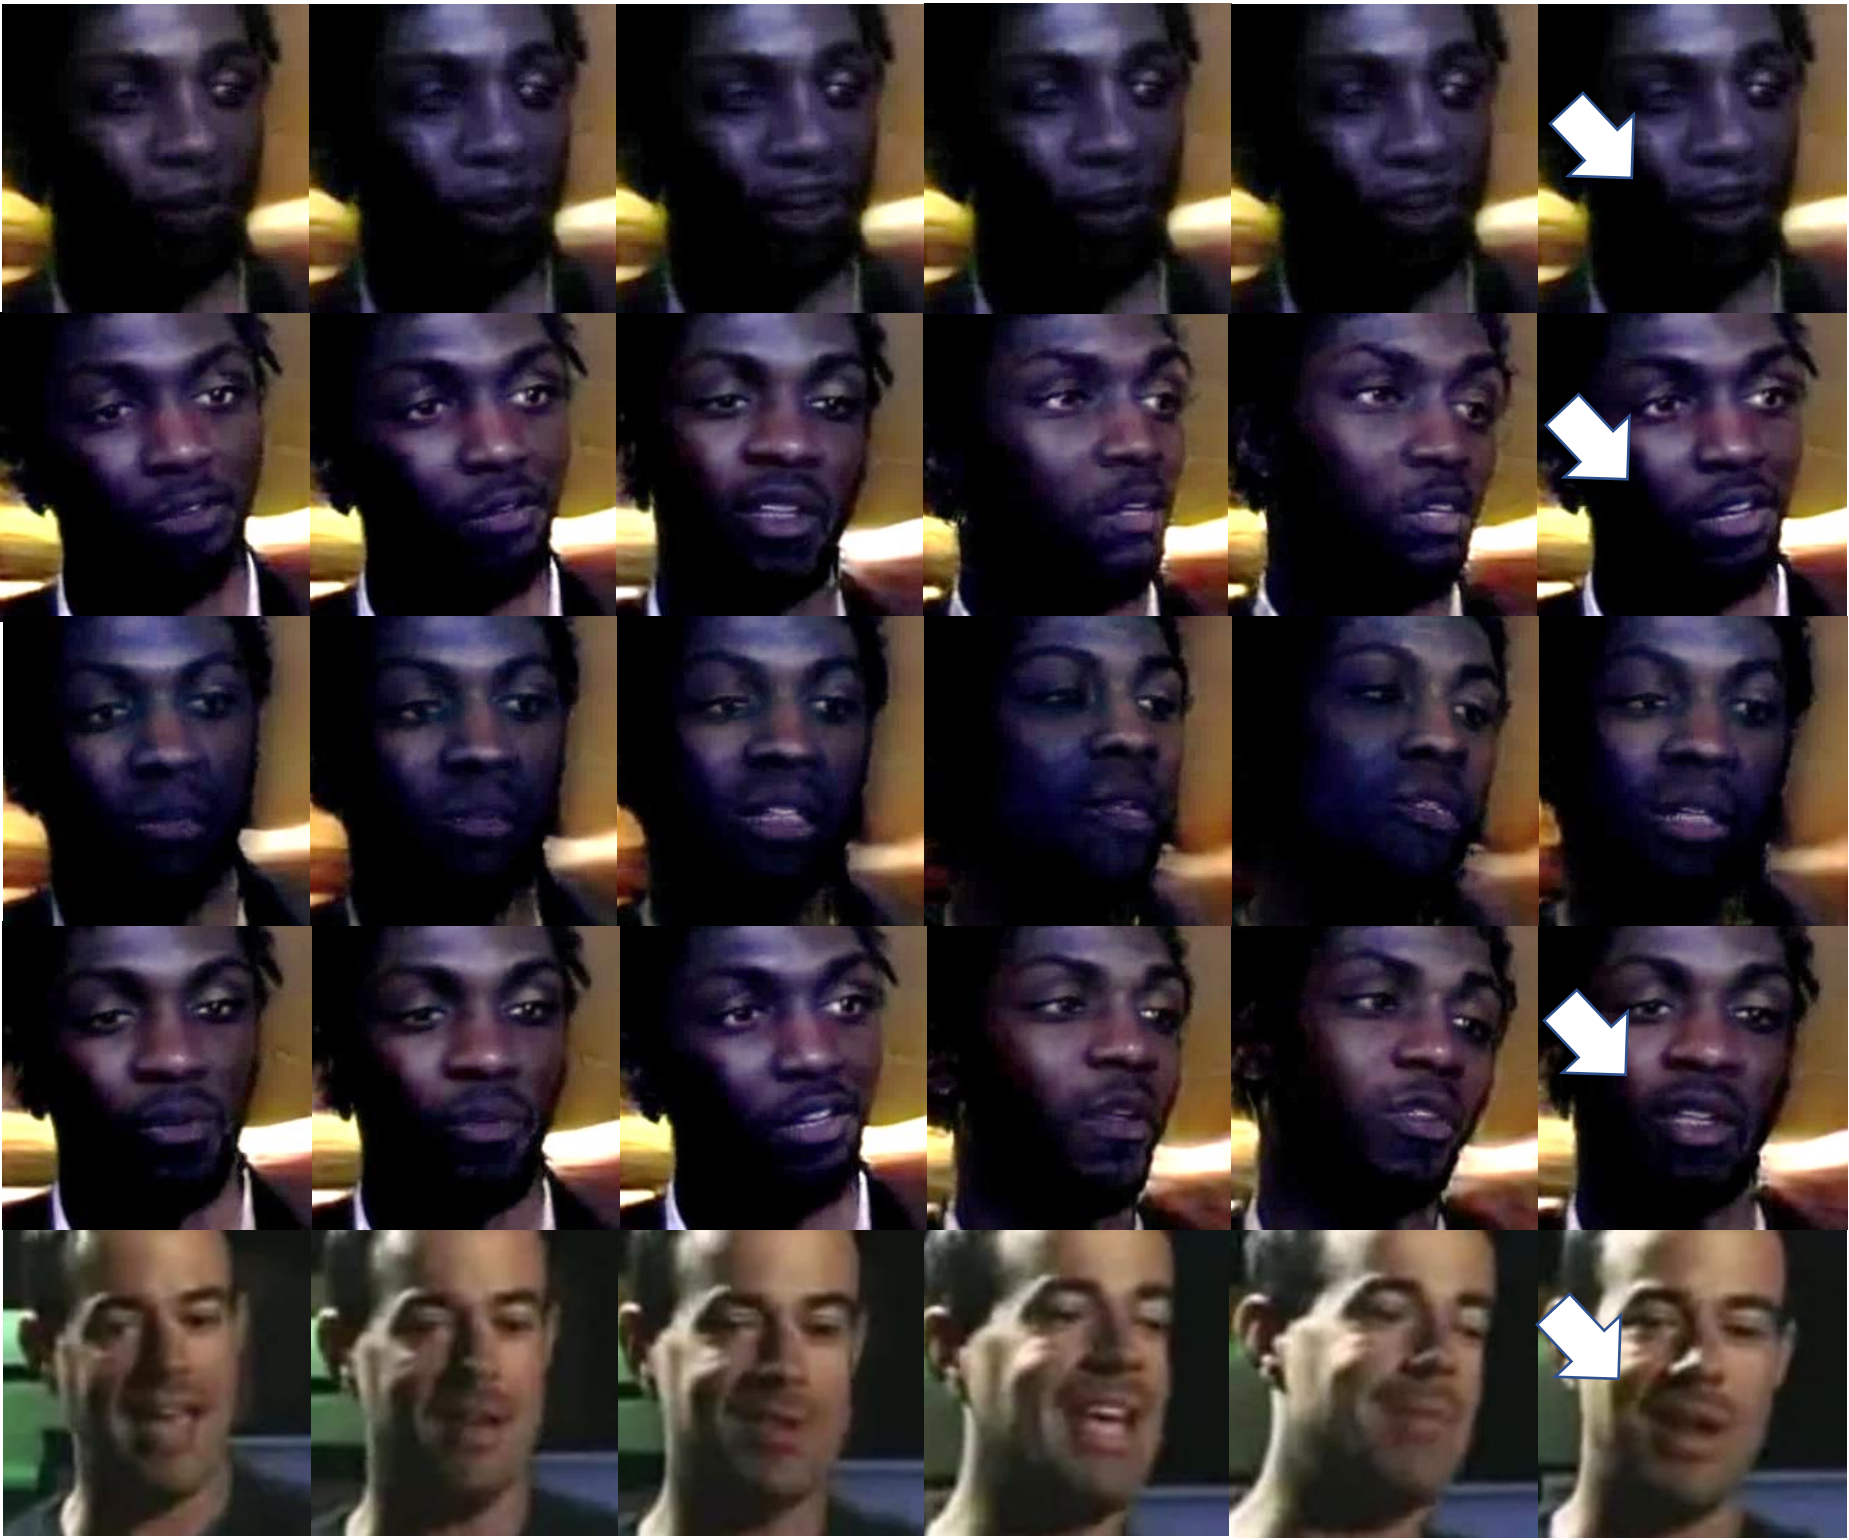

w/o  $\mathcal{L}_C$

Pose-dim  
36

AdaIN G

PC-AVS  
(Ours)

Pose  
Source
